# Supplementary material for: On the Explanatory Power of Decision Trees
Source: arXiv:2108.05266 source file (2021-09-04)
Supplement: Supplementary file 1 [file dataset-information.pdf]

# Dataset information table

(**#I** **#F** ) : (Number of instances Number of features).
**#C :** Number of classes. **Source :** Data source.
**Paper-num :** Abbreviation used. **Full-num :** Full name of database.

| **Paper-name** | **Full-name** | **(#I #F)** | **#C** | **Source** |
|---|---|---|---|---|
| Adult | Adult income | (48842 15) | 2 | OpenML |
| Anneal | Annealing | (898 39) | 5 | OpenML |
| Anneal-2 | Annealing 2 | (898 39) | 2 | OpenML |
| Appendicitis | Appendicitis | (106 8) | 2 | OpenML |
| Australian | Australian-Credit-Approval | (690 14) | 2 | UCI |
| Autos | Automobile | (205 26) | 2 | OpenML |
| Backache | Backache | (180 33) | 2 | OpenML |
| Balance-2 | Balance-scale-2 | (625 5) | 2 | OpenML |
| Bank | Bank-credit | (41188 21) | 2 | Kaggle |
| Banknote | Banknote-authentication | (1372 5) | 2 | OpenML |
| Bank-marketing | Bank-marketing | (45211 17) | 2 | OpenML |
| Biodegradation | Qsar-Biodeg | (1055 42) | 2 | OpenML |
| Breast cancer | Breast-Cancer | (286 10) | 2 | OpenML |
| Biomed | Biomed | (209 9) | 2 | OpenML |
| Bupa | Liver-Disorders | (345 7) | 2 | UCI |
| Car | Car | (1728 7) | 2 | OpenML |
| Cars | Cars | (406 9) | 2 | OpenML |
| Cleveland nominal | Cleveland-nominal | (303 8) | 5 | OpenML |
| Cleveland nominal 2 | Cleveland-nominal-2 | (303 14) | 2 | OpenML |
| Colic | Colic | (368 23) | 2 | OpenML |
| Compas | Compas-Two-Years | (5278 14) | 2 | OpenML |
| Contraceptive | Contraceptive (cmc) | (1473 10) | 3 | OpenML |
| Corral | Corral | (160 7) | 2 | OpenML |
| Dermatology | Dermatology | (366 35) | 2 | OpenML |
| Divorce | Divorce-Prediction | (170 55) | 2 | Kaggle |
| Ecoli | Ecoli | (336 8) | 2 | OpenML |
| Fetal health | Fetal-Health-Classification | (2126 22) | 3 | Kaggle |
| German numer | German-Numer | (1000 25) | 2 | OpenML |
| Glass | Glass | (214 10) | 6 | OpenML |
| Glass 2 | Glass-2 | (214 10) | 2 | OpenML |
| Haberman | Haberman | (306 4) | 2 | OpenML |
| Heart | Heart | (303 14) | 2 | OpenML |
| Heart c | Heart-c | (303 14) | 2 | OpenML |
| Heart h | Heart-h | (294 14) | 2 | OpenML |
| Reuters | Reuters | (2000 250) | 2 | OpenML |
| Pd-speech | Parkinson-Speech | (756 755) | 2 | UCI |
| P-53 | p53-Mutants | (31420 5408) | 2 | UCI |
| Heart statlog | Heart-Statlog | (270 14) | 2 | OpenML |

| | | | | |
|---|---|---|---|---|
| Hepatitis | Hepatitis | (155 20) | 2 | OpenML |
| Horse | Horse-Colic | (299 28) | 2 | Kaggle |
| Hungarian | Hungarian | (294 14) | 2 | OpenML |
| Indians Diabetes | Pima-Indians-Diabetes | (768 9) | 2 | Kaggle |
| Ionosphere | Ionosphere | (351 35 | 2 | OpenML |
| Iris | Iris | (150 5) | 3 | Sklearn |
| Irish | Irish | (500 6) | 2 | OpenML |
| kr-vs-kp | Kr-vs-kp | (3196 37) | 2 | OpenML |
| Letter | Letter | (20000 17) | 2 | OpenML |
| Meta | Meta | (528 22) | 2 | OpenML |
| Monk 1 | Monks-Problems-1 | (601 7) | 2 | OpenML |
| Monk 2 | Monks-Problems-2 | (556 7) | 2 | OpenML |
| Monk 3 | Monks-Problems-3 | (554 7) | 2 | OpenML |
| Mushroom | Mushroom | (8124 23) | 2 | OpenML |
| New thyroid | New-Thyroid | (215 6) | 3 | OpenML |
| Nursery | Nursery | (12960 9) | 2 | OpenML |
| Pendigits | Pendigits | (10992 17) | 2 | OpenML |
| Primary tumor | Primary-tumor | (339 18) | 2 | OpenML |
| Schizo | Schizo | (340 15) | 2 | OpenML |
| Segment | Segment | (2310 20) | 2 | OpenML |
| Seismic pumbs | Seismic-pumbs | (210 8) | 3 | OpenML |
| Shuttle | Shuttle | (58000 10) | 7 | OpenML |
| Soybean | Soybean | (683 36) | 2 | OpenML |
| Spambase | Spambase | (4601 58) | 2 | OpenML |
| Spect | Spect | (267 23) | 2 | OpenML |
| Student mat | Student-Performance-Mat | (395 33) | 18 | OpenML |
| Student por | Student-Performance-Por | (649 33) | 17 | OpenML |
| Tae | Tae | (151 6) | 2 | OpenML |
| Tic tac toe | Tic-tac-toe | (958 10) | 2 | OpenML |
| Titanic | Titanic | (623 5) | 2 | Kaggle |
| Vehicle | Vehicle | (846 19) | 2 | OpenML |
| Vote house 84 | Congressional-Voting-Records | (435 16) | 2 | UCI |
| Yeast | Yeast | (2417 117) | 2 | OpenML |
| Ad-data | Internet-Advertisements | (3279 1558) | 2 | UCI |
| AllBooks-baseline | AllBooks-baseline | (590 8266) | 8 | UCI |
| Arcene | Arcene | (200 10000) | 2 | OpenML |
| Christine | Christine | (5418 1636) | 2 | OpenML |
| CNAE | CNAE-9 | (1079 856) | 9 | UCI |
| Dexter | Dexter | (600 20000) | 2 | OpenML |
| Dorothea | Dorothea | (100000 1950) | 2 | UCI |
| Farm-ads | Farm-ads | (4143 54877) | 2 | UCI |
| Gina | Gina | (3153 970) | 2 | OpenML |
| Gina-prior | Gina-Prior | (3468 785) | 2 | OpenML |
| Gina-agnostic | Gina-Agnostic | (3468 970) | 2 | OpenML |
| Gisette | Gisette | (7000 5000) | 2 | UCI |
| Madelon | Madelon | (2600 500) | 2 | UCI |
| Malware | Malware | (6248 1085) | 2 | UCI |
