# Supplementary material for: On the Explanatory Power of Decision Trees
Source: arXiv:2108.05266 source file (2021-09-04)
Supplement: Supplementary file 2 [file full-proof-version.pdf]

# On Computing Short Reasons for Decision Trees

**Tracking Number: #3047**


## Abstract

Decision trees are popular ML models for the classification task because they are usually considered as highly interpretable. Indeed, for any instance to be classified using a decision tree, one can easily determine a subset of its features in order to explain the classification that is achieved. An irredundant subset of features, called a sufficient reason, can also be computed efficiently from the given instance. However, sufficient reasons are not guaranteed to be intelligible because they may contain too many features. In order to deal with this issue, we present a refinement and a generalization of the notion of sufficient reasons. We identify the complexity of computing such reasons for a given instance when the classifier is a decision tree, and we describe and evaluate algorithms for deriving them.


## 1 Introduction

In essence, explaining a decision to a person is to give the details or *reasons* that help the person understand why the decision has been made. This is a significant issue especially when decisions are made by Machine Learning (ML) models, such as random forests, Markov networks, support vector machines, and deep neural networks. Actually, with the growing number of applications that rely on ML techniques, researches on eXplainable AI (XAI) have become increasingly important, by providing efficient methods for interpreting ML models, and explaining their decisions (see for instance [Frosst and Hinton, 2017; Guidotti *et al.*, 2019; Hooker *et al.*, 2019; Huysmans *et al.*, 2011; Ignatiev *et al.*, 2019; Kim *et al.*, 2018; Lundberg and Lee, 2017; Miller, 2019; Molnar, 2019; Ribeiro *et al.*, 2016; Shih *et al.*, 2019]).

For classification problems, *decision trees* [Breiman *et al.*, 1984; Quinlan, 1986] are models of paramount importance in XAI, as they can be easily read by recursively breaking a choice into sub-choice until a decision is reached. Although there is no formal notion of *interpretability* [Lipton, 2018], decision trees are arguably among the most interpretable ML models, endowed with two key characteristics. On the one hand, decision trees are *transparent*: each node in a decision tree has some meaning, and the principles used for generating all nodes can be explained. On the other hand, decision trees are *locally explainable*: by construction of a decision tree, any input instance $\boldsymbol{x}$ is mapped to a unique root-to-leaf path $p$ that yields to a decision $y$. The subset of features occurring in $p$ can be viewed as a "direct reason" for classifying $\boldsymbol{x}$ as $y$. Because of their interpretability, decision trees are often considered are target models for distilling a black-box model into a comprehensible one [Breiman and Shang, 1996; Frosst and Hinton, 2017]. Furthermore, decision trees are often the components of choice for building (less interpretable, but potentially more accurate) ensemble classifiers, such as random forests [Breiman, 2001] and gradient boosted decision trees [Chen and Guestrin, 2016].

Although there is no consensus on what constitutes a "good" explanation [Narayanan *et al.*, 2018; Miller, 2019; Srinivasan and Chander, 2020], when it comes to explaining classification tasks, the notion of *sufficient reasons* [Darwiche and Hirth, 2020] (also known as prime implicant explanations [Shih *et al.*, 2018]) appears as a valuable candidate. A sufficient reason for an instance $\boldsymbol{x}$ classified as $y$ by a Boolean function $f$ is a subset $t$ of the features of $\boldsymbol{x}$ that is minimal with respect to set inclusion, and such that any instance $\boldsymbol{x}'$ sharing this set $t$ of features is also classified as $y$ by $f$. The significance of sufficient reasons comes from Occam's razor which roughly states that the best explanations are the simpler ones. Indeed, since any sufficient reason $t$ for is minimal w.r.t. set inclusion, it does not contain any locally irrelevant feature for classifying $\boldsymbol{x}$. In other words, if $t$ is a sufficient reason for an instance $\boldsymbol{x}$, labeled as $y$ by the classifier $f$, then removing any feature from $t$ would call into question the fact that $\boldsymbol{x}$ is classified as $y$ by $f$.

When the Boolean function $f$ is represented by a decision tree, say $T$, the direct reason $p$ obtained by reading the root-to-leaf path that classifies the input instance $\boldsymbol{x}$ contains typically far less features than $\boldsymbol{x}$ itself. However, from the theory side, it has been shown recently that $p$ may contain arbitrarily many more features than a sufficient reason for $\boldsymbol{x}$ given $T$ [Izza *et al.*, 2020]. Furthermore, from a more practical side, experiments reported in the same paper have pointed out that the number of extra features contained in direct reasons can be significantly larger than the size of sufficient reasons. Fortunately, one can take advantage of a greedy strategy to eliminate efficiently from $p$ any irrelevant feature, and this results in a polynomial-time algorithm for computing a sufficient reason for $\boldsymbol{x}$ given $T$.

Does this mean that the game is over and the question of explaining predictions from decision trees fully addressed? Not really: it cannot be guaranteed that the sufficient reasons computed by the greedy strategy are intelligible enough, because they may contain (too) many features. To this very point, it must be kept in mind that explaining is a social process [Miller, 2019], where explainees are *human beings*, who (inherently) have *cognitive limitations*. In his seminal paper [Miller, 1956], Psychologist George Miller introduced the idea of people "chunking" items (i.e., grouping them together as a unit) and argued that due to human memory limitations, the size of chunks is limited to 7, plus or minus 2. Ever since then, many experiments in cognitive science have confirmed this limitation. Restricting explanations to contain only few features thus appears as an important requirement for ensuring that they are intelligible. So, what can be done if the sufficient reason that has been computed includes too many attributes for being considered as intelligible? As a step towards more intelligibility, is it possible to define well-founded notions of reasons requiring less attributes than sufficient reasons?

These are the main research questions considered in the paper. In order to go even further in the direction of characterizing and computing simple explanations, we first consider a refinement of the notion of sufficient reasons, namely *minimal reasons*, that focuses on explanations of minimal size. We also consider a generalization of sufficient reasons, namely *probable reasons*, for which a small proportion of models can disagree with the classification made on the input instance. In both cases, we identify the complexity of computing a reason for a given instance when the classifier is a decision tree, and we describe exact or approximate algorithms for deriving such reasons. Finally, we report empirical results illustrating, from a practical viewpoint, the gain in intelligibility that is obtained via minimal reasons and probable reasons, and the performances of the algorithms for computing them.

The paper is organized as follows. Preliminaries about decision trees and sufficient reasons are given in Section 2. Minimal and probable reasons are defined and analyzed in Section 3. Experimental results are reported in Section 4. Finally, Section 5 concludes the paper. Proofs and detailed empirical results are provided as a supplementary material.

## 2 Decision Trees and Sufficient Reasons

For an integer $n$, let $[n]$ be the set $\{1, \cdots, n\}$. By $\mathcal{F}_n$ we denote the class of all Boolean functions from $\{0,1\}^n$ to $\{0,1\}$, and we use $X_n = \{x_1, \cdots, x_n\}$ to denote the set of input Boolean variables. Any assignment $\boldsymbol{x} \in \{0,1\}^n$ is called an *instance*. If $f(\boldsymbol{x}) = 1$ for some $f \in \mathcal{F}_n$, then $\boldsymbol{x}$ is called a *model* of $f$. We refer to $f$ as a propositional formula when it is described using the Boolean connectives $\wedge$ (conjunction), $\vee$ (disjunction) and $\neg$ (negation), together with the Boolean constants 1 (true) and 0 (false). As usual, a *literal* $l_i$ is a variable $x_i$ or its negation $\neg x_i$, also denoted $\overline{x}_i$. A *term* (or *monomial*) $t$ is a conjunction of literals, and a *clause* $c$ is a disjunction of literals. A $\texttt{DNF}$ *formula* is a disjunction of terms and a $\texttt{CNF}$ *formula* is a conjunction of clauses.

In what follows, we shall often treat assignments as terms, and (consistent) terms as sets of literals. Given an assignment $\boldsymbol{z} \in \{0,1\}^n$, the corresponding term is defined as

$$t_{\boldsymbol{z}} = \bigwedge_{i=1}^{n} x_i^{z_i} \text{ where } x_i^0 = \overline{x}_i \text{ and } x_i^1 = x_i$$

A term $t$ *covers* an assignment $\boldsymbol{z}$ if $t \subseteq t_{\boldsymbol{z}}$. An *implicant* of a Boolean function $f$ is a term that implies $f$, that is, a term $t$ such that $f(\boldsymbol{z}) = 1$ for every assignment $\boldsymbol{z}$ covered by $t$. A *prime implicant* of $f$ is an implicant $t$ of $f$ such that no proper subset of $t$ is an implicant of $f$.

With these basic notions in hand, we shall focus on the following representation class of Boolean functions:

**Definition 1** (Decision Tree)**.** *A (Boolean)* decision tree *is a binary tree $T$, each of whose internal nodes is labeled with one of $n$ input Boolean variables, and whose leaves are labeled* 0 *or* 1*. Every variable is assumed (without loss of generality) to appear at most once on any root-to-leaf path (read-once property). The value $T(\boldsymbol{x}) \in \{0,1\}$ of $T$ on an input instance $\boldsymbol{x}$ is given by the label of the leaf reached from the root as follows: at each node, go to the left or right child depending on whether the input value of the corresponding variable is* 0 *or* 1*, respectively. The size of $T$, denoted $|T|$, is given by the number of its nodes.*

The class of decision trees over $X_n$ is denoted $\texttt{DT}_n$. It is well-known that any decision tree $T \in \texttt{DT}_n$ can be transformed in linear time into an equivalent disjunction of terms, denoted $\texttt{DNF}(T)$, where each term corresponds to a path from the root to a leaf labeled with 1. Dually, $T$ can be transformed in linear time into a conjunction of clauses, denoted $\texttt{CNF}(T)$, where each clause is the negation of the term describing a path from the root to a leaf labeled with 0.

For illustration, the following toy example will be used throughout the paper as a running example:

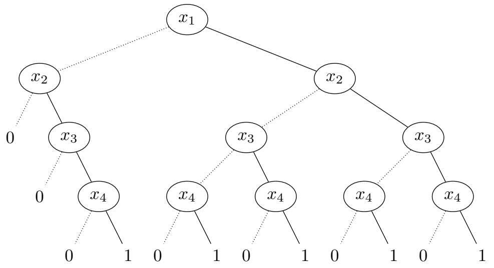


Figure 1: A decision tree $T$ for recognizing *Cattleya* orchids. The left (resp. right) child of any decision node labelled by $x_i$ corresponds to the assignment of $x_i$ to 0 (resp. 1).

**Example 1.** *The decision tree in Figure 1 separates Cattleya orchids from other orchids using the following features:*

- $x_1$*: "has fragrant flowers";*
- $x_2$*: "has one or two leaves";*
- $x_3$*: "has large flowers";*
- $x_4$*: "is sympodial";*
- $x_5$*: "has white flowers".*

*By construction, $\overline{x}_1 \wedge x_2 \wedge x_3 \wedge x_4$ is a term of* $\texttt{DNF}(T)$*, and $x_1 \vee x_2$ is a clause of* $\texttt{CNF}(T)$*. Note that $x_5$ is a (globally) irrelevant feature since it does not appear in any path of $T$.*

The key focus of this study is to explain *why* a decision tree $T \in \texttt{DT}_n$ classifies an incoming instance $\boldsymbol{x}$ as positive. A *reason* for $T(\boldsymbol{x}) = 1$ typically takes the form of conjunction of literals which together justify the prediction made by $T$ on $\boldsymbol{x}$. We mention in passing that focusing on the case $T(\boldsymbol{x}) = 1$ is without any loss of generality because $\texttt{DT}_n$ is closed under negation.[1] As a salient characteristic, decision trees convey a single explicit explanation for classifying any input instance:

**Definition 2** (Direct Reason). *Let $T \in \texttt{DT}_n$ and $\boldsymbol{x} \in \{0,1\}^n$ such that $T(\boldsymbol{x}) = 1$. The* direct reason *for $\boldsymbol{x}$ given $T$ is the term, denoted $p^T_{\boldsymbol{x}}$, corresponding to the unique root-to-leaf path of $T$ that is compatible with $\boldsymbol{x}$.*

**Example 2.** *Based on our running example, we can observe that $T(\boldsymbol{x}) = 1$ for the instance $\boldsymbol{x} = (1, 1, 1, 1, 1)$. The direct reason for $\boldsymbol{x}$ given $T$ is the term $p^T_{\boldsymbol{x}} = x_1 \wedge x_2 \wedge x_3 \wedge x_4$.*

Another important notion when dealing with the explanation of predictions is the following:

**Definition 3** (Sufficient Reason). *Let $f \in \mathcal{F}_n$ and $\boldsymbol{x} \in \{0,1\}^n$ such that $f(\boldsymbol{x}) = 1$. A* sufficient reason *for $\boldsymbol{x}$ given $f$ is a prime implicant $t$ of $f$ that covers $\boldsymbol{x}$.*

**Example 3.** *In our running example, $x_2 \wedge x_3 \wedge x_4$ is a sufficient reason for $\boldsymbol{x}$ given $T$. It is a better explanation than the direct reason $p^T_{\boldsymbol{x}} = x_1 \wedge x_2 \wedge x_3 \wedge x_4$, since $x_1$ is redundant (locally irrelevant) in the direct reason for $\boldsymbol{x}$.*

For the class $\texttt{DT}_n$, it is already known that sufficient reasons can be found in polynomial time (see e.g., [Izza *et al.*, 2020]). More precisely, given $T \in \texttt{DT}_n$ and $\boldsymbol{x} \in \{0,1\}^n$ such that $T(\boldsymbol{x}) = 1$, one can return in $\mathcal{O}(|T|n)$ time a sufficient reason $t$ for $\boldsymbol{x}$ given $T$ using the following greedy algorithm (that is reminiscent to the one considered in [Schrag, 1996] for a knowledge compilation purpose): start with $t = t_{\boldsymbol{x}}$, and iterate over the literals $l_i$ of $t$ by checking whether $t$ deprived of $l_i$ is an implicant of $T$.[2] If so, remove $l_i$ from $t$ and proceed to the next literal. Once all literals in $t_{\boldsymbol{x}}$ have been examined, the final term $t$ is by construction an implicant of $T$ such that removing any literal from it would lead to a term that is not any longer an implicant of $T$. Thus, $t$ is a prime implicant of $T$ containing only literals from $\boldsymbol{x}$. Clearly enough, instead of starting the greedy algorithm with $t = t_{\boldsymbol{x}}$, one may consider any implicant of $T$ that covers $\boldsymbol{x}$. In particular, the greedy algorithm can be run on $t = p^T_{\boldsymbol{x}}$.

# 3 Beyond Sufficient Reasons

## 3.1 Minimal Reasons

Since conciseness is often a desirable property of explanations, a natural way for improving the clarity of sufficient reasons is to focus on the shortest ones:

**Definition 4** (Minimal Reason). *Let $f \in \mathcal{F}_n$ and $\boldsymbol{x} \in \{0,1\}^n$ such that $f(\boldsymbol{x}) = 1$. A* minimal reason *for $\boldsymbol{x}$ given $f$ is a sufficient reason for $\boldsymbol{x}$ given $f$ that contains a minimal number of literals.*

[1]For any $T \in \texttt{DT}_n$, $\neg T$ is obtained by just replacing from $T$ the label of each leaf with its complement. So, a reason why $T(\boldsymbol{x}) = 0$ is precisely the same as a reason why $(\neg T)(\boldsymbol{x}) = 1$.

[2]This can be done in $O(|T|)$ time by checking whether $t \setminus \{l_i\}$ is an implicant of $\texttt{CNF}(T)$.

**Example 4.** *Based on our running example, $x_1 \wedge x_4$ is a minimal reason for $\boldsymbol{x}$ given $T$, while $x_2 \wedge x_3 \wedge x_4$ is not.*

Importantly, *minimal reasons* should not to be confused with *minimum-cardinality explanations* [Shih *et al.*, 2018], where the minimality condition bears on the features set to 1 in the input instance. In fact, as a direct by-product of Proposition 8 from [Audemard *et al.*, 2020], computing a minimum-cardinality explanation for an input instance $\boldsymbol{x}$ given a decision tree $T$ can be done in polynomial-time. Unfortunately, this is not the case for minimal reasons, which are computationally more demanding:

**Proposition 1.** *Let $T \in \texttt{DT}_n$ and $\boldsymbol{x} \in \{0,1\}^n$ such that $T(\boldsymbol{x}) = 1$. Computing a minimal reason for $\boldsymbol{x}$ given $T$ is* NP*-hard.*

A source of complexity that may explain this hardness result is the number of sufficient reasons for an input instance $\boldsymbol{x}$, which can be exponential in the size of the decision tree at hand. Indeed, even for the restricted class of decision trees with logarithmic depth, an input instance can have exponentially many sufficient reasons:

**Proposition 2.** *There is a decision tree $T \in \texttt{DT}_n$ of depth $\log_2(n+1)$ such that for any $\boldsymbol{x} \in \{0,1\}^n$, the number of sufficient reasons for $\boldsymbol{x}$ given $T$ is at least $\lfloor \frac{3}{2}^{\frac{n+1}{2}} \rfloor$.*

A common approach for handling NP-optimization problems is to rely on modern constraint solvers. One follows this direction here and casts the task of finding minimal reasons as a Boolean constraint optimization problem. We first need to recall that a PARTIAL MAXSAT problem consists of a pair $(C_{\text{soft}}, C_{\text{hard}})$ of CNF formulae, and the goal is to find a Boolean assignment that satisfies a maximum number of clauses in $C_{\text{soft}}$, while satisfying all clauses in $C_{\text{hard}}$.

**Proposition 3.** *Let $T$ be a decision tree in $\texttt{DT}_n$ and $\boldsymbol{x} \in \{0,1\}^n$ be an instance such that $T(\boldsymbol{x}) = 1$. Let $(C_{\text{soft}}, C_{\text{hard}})$ be an instance of the* PARTIAL MAXSAT *problem such that:*

$$C_{\text{soft}} = \{\overline{x}_i : x_i \in t_{\boldsymbol{x}}\} \cup \{x_i : \overline{x}_i \in t_{\boldsymbol{x}}\}$$
$$C_{\text{hard}} = \{c_{|\boldsymbol{x}} : c \in \texttt{CNF}(T)\}$$

*where $c_{|\boldsymbol{x}} = c \cap t_{\boldsymbol{x}}$ is the restriction of $c$ to the literals in $t_{\boldsymbol{x}}$. Any optimal solution of $(C_{\text{hard}}, C_{\text{soft}})$ is a minimal reason for $\boldsymbol{x}$ given $T$.*

As an alternative to PARTIAL MAXSAT solving, we may explore the possibility of finding good approximations of minimal reasons in polynomial-time. For decision trees, this task can be cast as a MIN HITTING SET problem: given a representation $T \in \texttt{DT}_n$ and an instance $\boldsymbol{x} \in \{0,1\}^n$ such that $T(\boldsymbol{x}) = 1$, let $H_{\boldsymbol{x}}(T)$ be the hypergraph formed by the set of vertices $t_{\boldsymbol{x}}$ and the set of hyperedges $\{c_{|\boldsymbol{x}} : c \in \texttt{CNF}(T)\}$. By construction, $t$ is a minimal reason for $\boldsymbol{x}$ given $T$ if and only if $t$ is a minimal hitting set of $H_{\boldsymbol{x}}(T)$. Based on this equivalence, the task of finding minimal reasons can be approximated using the following *greedy covering algorithm*: starting from $t = \varnothing$, iteratively add to $t$ a vertex $l_i \in t_{\boldsymbol{x}}$ of maximal degree, and removes it together with all adjacent hyperedges in $H_{\boldsymbol{x}}(T)$. Based on the performance analysis of the greedy covering algorithm [Slavík, 1997], the size of the

final term $t$ is at most $\ln n - \ln\ln n + 0.78$ larger than the size of a minimal reason for $\boldsymbol{x}$ given $T$. To sum up:

**Proposition 4.** *Let $T \in \mathtt{DT}_n$, and $\boldsymbol{x} \in \{0,1\}^n$ such that $T(\boldsymbol{x}) = 1$. Computing a minimal reason for $\boldsymbol{x}$ given $T$ is approximable to within a ratio of* $\ln n - \ln\ln n + \Theta(1)$.

### 3.2 Probable Reasons

A natural way to circumvent the computational barrier of finding minimal reasons is to rely on a probabilistic notion of prime implicant explanations, as suggested in [Wäldchen *et al.*, 2019]. This leads to generalize the notion of sufficient reasons, instead of refining it.

Basically, the idea of "probable‘" prime implicants stems from the fact that standard, "logical" prime implicants are often too rigid for high dimensional, and possibly noisy, classification tasks. Thus, by forgetting few models of the classifier $f$, probable prime implicants may provide much shorter explanations. In formal terms, let $\mathbb{P}_{\boldsymbol{z}}[f(\boldsymbol{z})]$ be the probability that an assignment $\boldsymbol{z}$, drawn at random according to the uniform distribution over $\{0,1\}^n$, is a model of $f$, i.e.

$$\mathbb{P}_{\boldsymbol{z}}[f(\boldsymbol{z})] = \frac{|\boldsymbol{z} \in \{0,1\}^n : f(\boldsymbol{z}) = 1|}{|\boldsymbol{z} \in \{0,1\}^n|}$$

Now, let $\mathbb{P}_{\boldsymbol{z}}[f(\boldsymbol{z}) \mid t \subseteq t_{\boldsymbol{z}}]$ be the conditional probability that a random assignment $\boldsymbol{z}$ is a model of $f$, given that $\boldsymbol{z}$ is an extension of $t$:

$$\mathbb{P}_{\boldsymbol{z}}[f(\boldsymbol{z}) \mid t \subseteq t_{\boldsymbol{z}}] = \frac{|\boldsymbol{z} \in \{0,1\}^n : f(\boldsymbol{z}) = 1 \text{ and } t \subseteq t_{\boldsymbol{z}}|}{|\boldsymbol{z} \in \{0,1\}^n : t \subseteq t_{\boldsymbol{z}}|}$$

For a confidence parameter $\delta \in [0,1]$, a term $t$ is called a *$\delta$-probable implicant* of $f$ if $\mathbb{P}_{\boldsymbol{z}}[f(\boldsymbol{z}) \mid t \subseteq t_{\boldsymbol{z}}] \geq \delta$, that is, the proportion of extensions of $t$ that are models of $f$ is at least $\delta$. If $t$ is a $\delta$-probable implicant of $f$ and no proper subset of $t$ is a $\delta$-probable implicant of $f$, then $t$ is called a *$\delta$-probable prime implicant* of $f$. We are now in position to define $\delta$-probable reasons:

**Definition 5** ($\delta$-Probable Reason)**.** *Let $f \in \mathcal{F}_n$ and $\boldsymbol{x} \in \{0,1\}^n$ such that $f(\boldsymbol{x}) = 1$. A $\delta$-*probable reason *for $\boldsymbol{x}$ given $f$ is a $\delta$-probable prime implicant $t$ of $f$ such that $t \subseteq t_{\boldsymbol{x}}$.*

**Example 5.** *Based on our running example, we can observe that $x_2 \wedge x_4$ is not a sufficient reason for $\boldsymbol{x}$ given $T$, but it is still a $75\%$-probable reason for $\boldsymbol{x}$ (given $T$).*

Interestingly, computing a $\delta$-probable reason for $\boldsymbol{x}$ given a decision tree $T$ is tractable by slightly modifying the greedy algorithm used to find sufficient reasons. Namely, at each iteration $i \in [n]$, instead of checking whether the current term $t$, deprived from the literal $l_i$, is an implicant of $T$, we check whether $t \setminus \{l_i\}$ is a $\delta$-probable implicant of $T$. Using the fact that conditioning and model counting operations can be done in linear time for decision trees [Koriche *et al.*, 2013], the inequality $\mathbb{P}_{\boldsymbol{z}}[f(\boldsymbol{z}) \mid t \subseteq t_{\boldsymbol{z}}] \geq \delta$ can be checked in linear time. In a nutshell:

**Proposition 5.** *Let $T \in \mathtt{DT}_n$ and $\boldsymbol{x} \in \{0,1\}^n$ such that $T(\boldsymbol{x}) = 1$. Computing a $\delta$-probable reason for $\boldsymbol{x}$ given $T$ can be done in $O(n|T|)$ time.*

## 4 Experiments

We have performed a number of experiments in order (i) to evaluate the practical performance of the algorithms for computing sufficient, minimal and $\delta$-probable reasons, and (ii) to assess the gain in intelligibility that results from focusing on the size of these different reasons, relatively to the size of direct reasons.

### 4.1 Empirical setting

We have considered 90 datasets, which are standard benchmarks from the well-known repositories Kaggle[3], OpenML[4], and UCI[5]. Due to space constraints, the complete list of benchmarks used is reported as a supplementary material, together with additional information about the decision trees and the sizes of the different reasons that have been computed. Several datasets considered in our experiments include a large number of instances with a large number of features. Because some datasets are suited to the multi-label classification task, we used the standard "one versus all" policy to deal with them: all the classes but the target one are considered as the complementary class of the target. Categorical features have been treated as arbitrary numbers (the scale is nominal). As to numeric features, no data preprocessing has taken place: these features have been binarized on-the-fly by the decision tree learning algorithm that has been used.

For every benchmark $b$, a 10-fold cross validation process has been achieved. Namely, a set of 10 decision trees $T_b$ have been computed and evaluated from the labelled instances of $b$, partitioned into 10 parts. One part was used as the test set and the remaining 9 parts as the training set for generating a decision tree. This tree is thus in 1-to-1 correspondence with the test set chosen within the whole dataset $b$. The classification performance for $b$ was measured as the mean accuracy obtained over the 10 decision trees generated from $b$. For the decision tree learner, we have used the CART algorithm, and more specifically its implementation provided by the Scikit-Learn[6] library. All hyper-parameters of the learning algorithm have been set to their default value. Notably, decision trees have been learned using the Gini criterion, and without any maximal depth or any other manual limitation.

For each benchmark $b$, each decision tree $T_b$, and each instance $\boldsymbol{x}$ of the corresponding test set, we computed the direct reason for $\boldsymbol{x}$ given $T_b$, a sufficient reason for $\boldsymbol{x}$ given $T_b$, a minimal reason for $\boldsymbol{x}$ given $T_b$, and $\delta$-probable reasons for $\boldsymbol{x}$ given $T_b$ for several values of $\delta$ (95%, 90%, 75%). The sufficient reason and the $\delta$-probable reasons were computed from the direct reason. For computing minimal reasons, we used the Pysat[7] library, which provides the implementation of the RC2 Partial MaxSAT solver. This solver was run using the parameters corresponding to the "Glucose" setting. For each instance in a dataset and each type of reason, we computed the mean size of the reason (given as a number of binary features), together with the corresponding standard deviation.

[3] www.kaggle.com

[4] www.openml.org

[5] archive.ics.uci.edu/ml/

[6] scikit-learn.org/stable/index.html

[7] https://pysathq.github.io/

| Dataset | #I | #F | %A | #N | #MD | #B | #DR | #SR | #MR | #95-PR | #90-PR | #75-PR |
|---|---|---|---|---|---|---|---|---|---|---|---|---|
| Ad-data | 3279 | 1558 | 96.58 | 321.4 | 85.2 | 141.1 | 33.8±14.9 | 30.3±10.7 | 28.8±9.9 | 29.5±10.5 | 28.3±10.2 | 22.0±7.8 |
| Adult | 48842 | 14 | 81.41 | 12926.0 | 47.4 | 2973.2 | 17.4±5.9 | 16.5±5.1 | 16.5±5.1 | 16.3±5.2 | 15.7±5.1 | 12.9±4.5 |
| AllBooks | 590 | 8266 | 71.02 | 183.4 | 42.9 | 88.8 | 15.0±13.5 | 14.1±12.1 | 14.1±12.1 | 13.9±11.8 | 13.8±11.7 | 13.1±11.3 |
| Arcene | 200 | 10000 | 73.00 | 24.4 | 5.3 | 11.7 | 4.1±0.9 | 4.1±0.9 | 4.1±0.9 | 4.0±0.9 | 3.9±0.9 | 2.9±1.0 |
| Christine | 5418 | 1636 | 62.77 | 839.0 | 34.3 | 419.0 | 16.1±9.1 | 15.8±9.1 | 15.8±9.1 | 15.8±9.1 | 15.7±9.1 | 14.2±9.2 |
| CNAE | 1079 | 856 | 86.00 | 278.6 | 52.5 | 113.9 | 14.5±13.7 | 13.7±12.5 | 13.7±12.5 | 13.7±12.5 | 13.7±12.4 | 13.2±12.2 |
| Dexter | 600 | 20000 | 86.50 | 73.4 | 12.7 | 36.2 | 7.2±2.8 | 6.9±2.8 | 6.9±2.8 | 6.7±2.7 | 6.5±2.7 | 5.4±2.7 |
| Dorothea | 1150 | 100000 | 90.70 | 65.2 | 18.8 | 32.1 | 16.7±3.9 | 16.6±4.2 | 16.6±4.2 | 16.4±4.2 | 16.4±4.3 | 14.8±4.1 |
| Farm-ads | 4143 | 54877 | 86.75 | 543.2 | 91.3 | 264.6 | 25.9±21.4 | 24.7±20.6 | 24.7±20.6 | 24.2±20.6 | 23.6±20.4 | 21.1±19.8 |
| Gina | 3153 | 970 | 87.54 | 330.8 | 24.0 | 164.5 | 14.4±6.4 | 14.3±6.5 | 14.3±6.5 | 14.2±6.5 | 14.1±6.6 | 12.5±6.5 |
| Gina-p | 3168 | 970 | 86.77 | 375.4 | 21.1 | 186.7 | 13.4±4.7 | 13.3±4.7 | 13.2±4.7 | 13.2±4.7 | 13.1±4.8 | 11.5±4.6 |
| Gina-a | 3468 | 784 | 85.29 | 373.4 | 24.6 | 186.0 | 13.9±5.9 | 13.8±6.0 | 13.8±6.0 | 13.7±6.1 | 13.7±6.1 | 12.2±6 |
| Gisette | 7000 | 5000 | 93.67 | 347.6 | 36.0 | 173.3 | 25.2±10.4 | 25.0±10.5 | 25.0±10.5 | 25.0±10.5 | 24.8±10.6 | 2.6±10.7 |
| Madelon | 2600 | 500 | 76.00 | 365.8 | 17.6 | 181.9 | 10.6±3.5 | 10.4±3.6 | 10.4±3.6 | 10.4±3.6 | 10.3±3.6 | 8.9±3.7 |
| Malware | 6248 | 1084 | 99.09 | 88.0 | 11.1 | 43.0 | 7.3±1.6 | 7.1±1.4 | 7.1±1.4 | 6.7±1.4 | 6.4±1.3 | 4.9±1.2 |
| p53mutant | 31420 | 5407 | 99.36 | 171.2 | 38.9 | 85.1 | 37.4±4.7 | 37.4±4.8 | 37.4±4.8 | 37.4±4.8 | 37.4±4.8 | 35.4±4.8 |
| Pd-speech | 756 | 755 | 81.10 | 89.6 | 16.2 | 44.3 | 11.2±5.2 | 10.9±5.3 | 10.9±5.3 | 10.8±5.3 | 10.6±5.2 | 9.4±5.3 |
| Reuters | 2000 | 249 | 92.05 | 193.0 | 25.4 | 89.8 | 16.7±6.3 | 16.4±6.3 | 16.4±6.2 | 16.4±6.3 | 16.2±6.4 | 14.2±5.9 |
| Shuttle | 58000 | 9 | 99.98 | 65.6 | 9.0 | 32.3 | 7.2±1.7 | 7.2±1.7 | 7.2±1.7 | 7.2±1.7 | 7.2±1.7 | 6.2±1.6 |
| Spambase | 4601 | 58 | 92.05 | 530.4 | 32.3 | 261.1 | 15.9±6.3 | 15.3±6.1 | 15.4±6.1 | 14.9±6.1 | 14.5±6 | 11.9±5.4 |

Table 1: Results for 20 datasets. For each dataset, we indicate the number of instances (#I), the number of features (#F), the mean accuracy over the 10 decision trees (%A) that have been generated, the average number of nodes in those trees (#N), their maximal depth in average (#MD) the average number of binary features they are based on (#B). The average and standard deviation is provided for direct reasons (#DR), sufficient reasons (#SR), minimal reasons (#MR) and 95% / 90% / 75%-probable reasons (#95-PR / #90-PR / #75-PR).

In our experiments, we have also measured the runtimes required to compute any reason. All the experiments have been conducted on a computer equipped with Intel(R) Core(TM) i9-9900 CPU @ 3.10 GHz and 64 GiB of memory.

## 4.2 Results

Table 1 reports an excerpt of our results, focusing on 20 benchmarks out of 90 (the selected datasets are among those containing many instances and/or many features). The leftmost column gives the name of the dataset $b$, and the next two columns make precise its number of instances and its number of features. The four following columns are about the decision trees $T_b$ that have been learned, by indicating their mean accuracy, the average number of their nodes, their maximal depth in average, and the average number of binary features they are built on. The next columns give the results obtained for the direct reason, the sufficient reason, the minimal reason, the 95%-probable reason, the 90%-probable reason, and finally the 75%-probable reason. For each reason, we have reported its average size, together with its standard deviation.

In light of these results, we can observe that the direct reasons of input instances are typically far much shorter than the instances themselves. This is a strong argument about why decision trees are typically considered as interpretable models. Yet, when switching to the other types of reasons examined in the paper, some additional features are often removed. It is interesting to note that the reductions that are achieved (in number of literals) are more salient for the $\delta$-probable reasons (in particular, when $\delta = 75\%$) than for the minimal reasons. Empirically, it turns out that for many instances $\boldsymbol{x}$, the direct reason for $\boldsymbol{x}$ is actually a minimal reason, or an "almost minimal" one, in the sense that it contains very few irrelevant features for classifying $\boldsymbol{x}$. Though the suppression of irrelevant (or "probably irrelevant") features in reasons is not enough to guarantee that the size of the reasons will always stay below the cognitive barrier of $7 \pm 2$ features (as pointed out by George Miller), especially when dealing with high-dimensional classification tasks, this objective has been reached by the direct reasons for 68 out of 90 benchmarks used in the experiments.

In order to figure out the benefits obtained when switching from direct reasons to other reasons, we drew a number of scatter plots: each instance $\boldsymbol{x}$ of $b$ corresponds to a point, its $x$-coordinate gives the size of its direct reason, and its $y$-coordinate gives the size of the minimal reason (or of the 75%-probable reason) that has been computed. Figure 2 gives such scatter plots for the benchmarks "Add-data" and "Farm-ads". Here, we can observe that a significant reduction of the number of features used in the direct reasons may occur. Specifically, for minimal reasons, the average reduction of the size of the direct reasons achieved for "Add-data" (resp. "Farm-ads" ) was of 11.5% (resp. 3.5%) while the maximal reduction for "Add-data" (resp. "Farm-ads") was of 65.2% (resp. 76.2%). For 75%-probable reasons, the average reduction of the size of the direct reasons achieved for "Add-data" (resp. "Farm-ads") was of 32.9% (resp. 22%) while the maximal reduction for "Add-data" (resp. "Farm-ads") was of 100% (resp. 90%). Interestingly, for "Add-data", the sizes of minimal reasons (resp. 75%-probable reasons) never exceeded 37 (resp. 106) regardless of the size of direct reasons.

Finally, since the reduction of the size of the reasons achieved by considering 75%-probable reasons in comparison to direct reasons looked significant, we have also run additional experiments in order to get a clearer picture of the reduction that can be achieved when $\delta$ varies. We have computed the sizes of the $\delta$-probable reasons of instances while $\delta$ varies from 100% (in this case, $\delta$-probable reasons correspond to sufficient reasons) to 50%. Figure 3 reports such plots for the benchmarks "Madelon", "Malware", and "Spambase". As expected, one can observe that the mean size of the $\delta$-probable reasons smoothly decreases when $\delta$ diminishes.

As to the computation times, it turns out that all the algo-

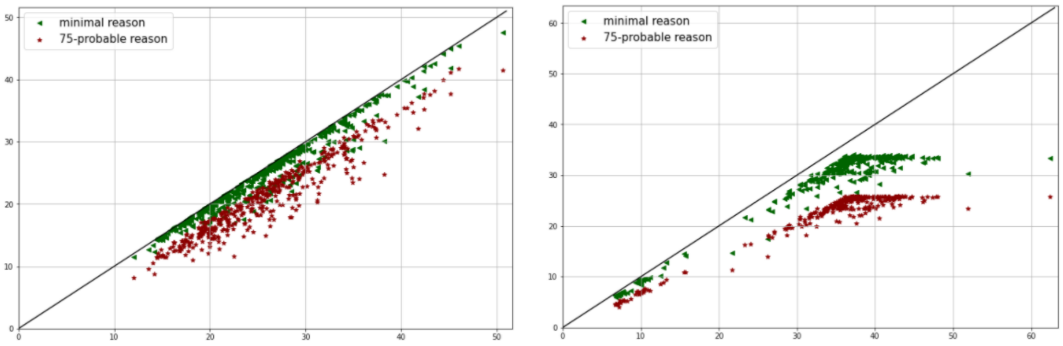


Figure 2: Comparison, for Farm-ads (left) and Ad-data (right), between the sizes of direct reasons vs. the sizes of minimal reasons (green triangles) and 75%-probable reasons (red stars).

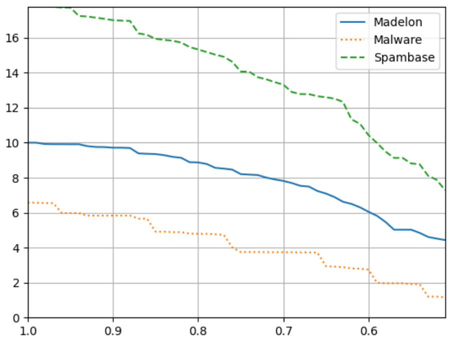


Figure 3: Average size of $\delta$-probable reasons when $\delta$ varies from 1 (sufficient reasons) to 0.5 for the datasets "Madelon", "Malware", and "Spambase".

rithms used for deriving reasons proved very efficient in practice (despite the use of a fully-interpreted version of Python for the implementation). Indeed, for every benchmark $b$ but "Adult", and every instance $\boldsymbol{x}$ of $b$, a reason for $\boldsymbol{x}$ given $T_b$ has been generated **in less than 100ms**, whatever the type of reason one was looking for. Note that "Adult" led to quite huge decision trees (in average, with 12926 nodes, based on more than 2973 binary features). Despite this size, for this dataset, the computation times for computing a reason never exceeded 600ms, except for minimal reasons which turned out to be more demanding from a computation point of view (as this was expected in light of Proposition 1). But it is worth noting that even the performance of the algorithm for computing minimal reasons was not that bad for this benchmark, with an average computation time of 2.69s and a maximal computation time of 5.06s. This explains why we have refrained from leveraging Proposition 4 to compute approximate minimal reasons.

## 5 Conclusion

It is acknowledged that intelligibility is among the research questions pertaining to XAI that have not been explored in depth, and that it should receive more attention [Doshi-Velez and Kim, 2017; Guidotti *et al.*, 2019]. Our work contributes to fill the gap, with a study of the intelligibility question for decision trees based on the sizes of the reasons.

Though it is possible to derive in polynomial time a sufficient reason for a given instance $\boldsymbol{x}$ when the classifier is a decision tree, we have argued that such a reason cannot be guaranteed as intelligible in the general case because it may contain too many features. In order to deal with this issue, we have focused on a refinement and on a generalization of the notion of sufficient reasons, namely the minimal reasons and the probable reasons, respectively. We have identified the complexity of computing such reasons for a given instance when the classifier is a decision tree, and we have described exact or approximate algorithms for deriving them. We have also presented empirical results for illustrating the gain in intelligibility minimal reasons and probable reasons may offer, as well as the performances of the algorithms that have been pointed out for computing them.

Interestingly, unlike direct reasons that are specific to decision trees, the notions of minimal reasons and of $\delta$-probable reasons make sense for any Boolean classifier (just as sufficient reasons do). Since, by construction, minimal reasons and $\delta$-probable reasons cannot be larger than sufficient reasons, they appear as valuable concepts to the purpose of getting more intelligible explanations for the classifications made. In the case of decision trees, all those reasons are in practice much smaller than the instances themselves. Though the most significant reduction w.r.t. the size of the instances is achieved by the direct reasons, our experiments revealed that some further reduction can take place when considering minimal reasons or $\delta$-probable reasons instead. In addition, in light of our experiments, the derivation of minimal reasons or of $\delta$-probable reasons does not require a tremendous computational effort. The reduction they can lead to is thus almost for free.

This work paves the way for some further developments. Identifying the complexity of deriving minimal reasons or $\delta$-probable reasons for other Boolean classifiers, and developing and evaluating algorithms to compute such reasons is is a perspective we will consider in the near future. Exploiting pieces of knowledge to simplify the reasons during their computation is another research direction we plan to follow.

## References


[Audemard *et al.*, 2020] G. Audemard, F. Koriche, and P. Marquis. On tractable XAI queries based on compiled representations. In *Proc. of KR'20*, pages 838–849, 2020.

[Breiman and Shang, 1996] L. Breiman and N. Shang. Born again trees. Technical report, https://www.stat.berkeley.edu/ breiman/BAtrees.pdf, 1996.

[Breiman *et al.*, 1984] L. Breiman, J. H. Friedman, R. A. Olshen, and C. J. Stone. *Classification and Regression Trees*. Wadsworth, 1984.

[Breiman, 2001] L. Breiman. Random forests. *Machine Learning*, 45(1):5–32, 2001.

[Chen and Guestrin, 2016] T. Chen and C. Guestrin. XGBoost: A scalable tree boosting system. In *Proc. of KDD'16*, page 785–794, 2016.

[Darwiche and Hirth, 2020] A. Darwiche and A. Hirth. On the reasons behind decisions. In *Proc. of ECAI'20*, pages 712–720, 2020.

[Doshi-Velez and Kim, 2017] F. Doshi-Velez and B. Kim. Towards a rigorous science of interpretable machine learning, 2017.

[Frosst and Hinton, 2017] N. Frosst and G. E. Hinton. Distilling a neural network into a soft decision tree. In *Proc. of the First International Workshop on Comprehensibility and Explanation in AI and ML*, volume 2071 of *CEUR Workshop Proceedings*. CEUR-WS.org, 2017.

[Guidotti *et al.*, 2019] R. Guidotti, A. Monreale, S. Ruggieri, F. Turini, F. Giannotti, and D. Pedreschi. A survey of methods for explaining black box models. *ACM Computing Surveys*, 51(5):93:1–93:42, 2019.

[Hooker *et al.*, 2019] S. Hooker, D. Erhan, P-J. Kindermans, and B. Kim. A benchmark for interpretability methods in deep neural networks. In *Proc. of NeurIPS'19*, pages 9737–9748, 2019.

[Huysmans *et al.*, 2011] J. Huysmans, K. Dejaeger, C. Mues, J. Vanthienen, and B. Baesens. An empirical evaluation of the comprehensibility of decision table, tree and rule based predictive models. *Decis. Support Syst.*, 51(1):141–154, 2011.

[Ignatiev *et al.*, 2019] A. Ignatiev, N. Narodytska, and J. Marques-Silva. Abduction-based explanations for machine learning models. In *Proc. of AAAI'19*, pages 1511–1519, 2019.

[Izza *et al.*, 2020] Y. Izza, A. Ignatiev, and J. Marques-Silva. On explaining decision trees. *CoRR*, abs/2010.11034, 2020.

[Karp, 1972] R.M. Karp. *Reducibility among combinatorial problems*, chapter Complexity of Computer Computations, pages 85–103. Plenum Press, New York, 1972.

[Kim *et al.*, 2018] B. Kim, M. Wattenberg, J. Gilmer, C. Cai, J. Wexler, F. Viegas, and R. Sayres. Interpretability beyond feature attribution: Quantitative testing with concept activation vectors (TCAV). In *Proc. of ICML'18*, pages 2668–2677, 2018.

[Koriche *et al.*, 2013] F. Koriche, J.-M. Lagniez, P. Marquis, and S. Thomas. Knowledge compilation for model counting: Affine decision trees. In *Proc. of IJCAI'13*, pages 947–953, 2013.

[Lipton, 2018] Z. C. Lipton. The mythos of model interpretability. *Communications of the ACM*, 61(10):36–43, 2018.

[Lundberg and Lee, 2017] S. Lundberg and S-I. Lee. A unified approach to interpreting model predictions. In I. Guyon, U. V. Luxburg, S. Bengio, H. Wallach, R. Fergus, S. Vishwanathan, and R. Garnett, editors, *Proc. of NIPS'17*, pages 4765–4774, 2017.

[Miller, 1956] G. A. Miller. The magical number seven, plus or minus two: Some limits on our capacity for processing information. *The Psychological Review*, 63(2):81–97, 1956.

[Miller, 2019] T. Miller. Explanation in artificial intelligence: Insights from the social sciences. *Artificial Intelligence*, 267:1–38, 2019.

[Molnar, 2019] Ch. Molnar. *Interpretable Machine Learning - A Guide for Making Black Box Models Explainable*. Leanpub, 2019.

[Narayanan *et al.*, 2018] M. Narayanan, E. Chen, J. He, B. Kim, S. Gershman, and F. Doshi-Velez. How do humans understand explanations from machine learning systems? an evaluation of the human-interpretability of explanation. *CoRR*, abs/1802.00682, 2018.

[Quinlan, 1986] J. R. Quinlan. Induction of decision trees. *Machine Learning*, 1(1):81–106, 1986.

[Ribeiro *et al.*, 2016] M. Ribeiro, S. Singh, and C. Guestrin. "Why should I trust you?": Explaining the predictions of any classifier. In *Proc. of KDD'16*, pages 97–101, 2016.

[Schrag, 1996] R. Schrag. Compilation for critically constrained knowledge bases. In *Proc. of AAAI'96*, pages 510–515, 1996.

[Shih *et al.*, 2018] A. Shih, A. Choi, and A. Darwiche. A symbolic approach to explaining Bayesian network classifiers. In *Proc. of IJCAI'18*, pages 5103–5111, 2018.

[Shih *et al.*, 2019] A. Shih, A. Darwiche, and A. Choi. Verifying binarized neural networks by Angluin-style learning. In *Proc. of SAT'19*, pages 354–370, 2019.

[Slavík, 1997] P. Slavík. A tight analysis of the greedy algorithm for set cover. *Journal of Algorithms*, 25(2):237 – 254, 1997.

[Srinivasan and Chander, 2020] R. Srinivasan and A. Chander. Explanation perspectives from the cognitive sciences - A survey. In *Proc. of IJCAI'20*, pages 4812–4818, 2020.

[Wäldchen *et al.*, 2019] S. Wäldchen, J. MacDonald, S. Hauch, and G. Kutyniok. The computational complexity of understanding network decisions. *CoRR*, abs/1905.09163, 2019.

# Proofs

## Proof of Proposition 1

*Proof.* We call MINIMAL REASON the problem that asks, given $T \in \mathtt{DT}_n$, $\boldsymbol{x} \in \{0,1\}^n$ with $T(x) = 1$ and $k \in \mathbb{N}$, whether there is an implicant $t$ of $T$ of size at most $k$ that covers $\boldsymbol{x}$.

Our objective is to prove that MINIMAL REASON is NP-hard. To this end, let us first recall that a *vertex cover* of an undirected graph $G = (X, E)$ is a subset $V \subseteq X$ of vertices such that $\{y, z\} \cap V \neq \varnothing$ for every edge $e = \{y, z\}$ in $E$. In the MIN VERTEX COVER problem, we are given a graph $G$ together with an integer $k \in \mathbb{N}$, and the task is to find a vertex cover $V$ of $G$ of size at most $k$. MIN VERTEX COVER is a well-known NP-hard problem [Karp, 1972], and we now show that it can be reduced in polynomial time to MINIMAL REASON.

Suppose that we are given a graph $G = (X, E)$ and assume, without loss of generality, that $G$ does not include isolated vertices. For any $y \in X$, let $E_y = \{e \in E : y \in e\}$ denote the set of edges in $G$ that are adjacent to $y$, and let $N_y = \{z \in X : \{y, z\} \in E\}$ denote the set of neighbors of $y$ in $G$. By $G \setminus y$, we denote the deletion of $y$ from $G$, obtained by removing $y$ and its adjacent edges, i.e., $G \setminus y = (X \setminus \{y\}, E \setminus E_y)$. We associate with $G$ a decision tree $T(G)$ over $X_n = X$ using the following recursive algorithm. If $G$ is the empty graph (i.e. $E = \varnothing$), then return the decision tree rooted at a 1-leaf. Otherwise, pick a node $y \in X$ and generate a decision tree $T(G)$ such that:

(1) the root is labeled by $y$;

(2) the left child is the decision tree encoding the monomial $\bigwedge N_y$;

(3) the right child is the decision tree $T(G')$ returned by calling the algorithm on $G' = G \setminus y$.

By construction, $T(G)$ is a complete backtrack search tree of the formula $\mathtt{CNF}(E) = \bigwedge\{(y \vee z) : \{y, z\} \in E\}$, which implies that $T(G)$ and $\mathtt{CNF}(E)$ are logically equivalent. Furthermore, $T(G)$ is a comb-shaped tree since recursion only on the rightmost branch. In particular, the algorithm runs in $\mathcal{O}(n|E|)$ time, since step (1) takes $\mathcal{O}(1)$ time, step (2) takes $\mathcal{O}(n)$ time, and step (3) is called at most $|E|$ times.

Now, with an instance $\boldsymbol{P}_1 = (G, k)$ of MIN VERTEX COVER, we associate the instance $\boldsymbol{P}_2 = (T(G), \boldsymbol{x}, k)$ of MINIMAL REASON, where $\boldsymbol{x} = (1, \cdots, 1)$. Based on the above algorithm, $\boldsymbol{P}_2$ can be constructed in time polynomial in the size of $\boldsymbol{P}_1$.

Let $V$ be a solution of $\boldsymbol{P}_1$. Since $V$ is a vertex cover of $G$, the term $t_V = \bigwedge V$ is an implicant of the formula $\mathtt{CNF}(E)$. Since $t_V \subseteq t_{\boldsymbol{x}}$ and $|t_V| \leq k$, it follows from the fact that $\mathtt{CNF}(E)$ and $T(G)$ are logically equivalent that $t_V$ is a solution of $\boldsymbol{P}_2$.

Conversely, let $t$ be a solution of $\boldsymbol{P}_2$. Since $t$ is an implicant of $T(G)$, it follows that $t$ is an implicant of $\mathtt{CNF}(E)$. This together with the fact that $t \subseteq t_{\boldsymbol{x}}$ implies that the subset of vertices $V \subseteq X_n$, satisfying $\bigwedge V = t$, is a vertex cover of $G$. Since $|V| \leq k$, it is therefore a solution of $\boldsymbol{P}_1$. □

## Proof of Proposition 2

*Proof.* Let $T$ be the complete binary tree of depth $k$, formed by $n = 2^k - 1$ internal nodes and $2^k$ leaves. We assume a breadth-first ordering of internal nodes, such that the root is labeled by $x_1$, the nodes of depth 1 are labeled by $x_2$ and $x_3$, and so on. For an arbitrary instance $\boldsymbol{x} \in \{0,1\}^n$ and any complete subtree $T'$ of $T$ of depth $d$, let $s(\boldsymbol{x}, T')$ denote the set of sufficient reasons of $\boldsymbol{x}$ given $T'$, and let $\sigma(\boldsymbol{x}, d) = |s(\boldsymbol{x}, T')|$ denote the number of those sufficient reasons. We show by induction on $d$ that:

$$\sigma(\boldsymbol{x}, 1) = 1 \tag{1}$$

$$\sigma(\boldsymbol{x}, d+1) = \sigma(\boldsymbol{x}, d)(\sigma(\boldsymbol{x}, d) + 1) \tag{2}$$

For the base case (1), any complete subtree $T'$ of $T$ of depth $d = 1$ has a single internal node, say $x_i$, with two leaves labeled by 0 and 1, respectively. Therefore, the unique sufficient reason for $\boldsymbol{x}$ given $T'$ is either $x_i$ or $\overline{x}_i$, and hence, $\sigma(\boldsymbol{x}, 1) = 1$. Now, consider any complete subtree $T'$ of $T$ of depth $d+1$ rooted at a node $x_i$. Let $T'_l(x_i)$ and $T'_r(x_i)$ denote the subtrees of depth $d$, respectively rooted at the left child of $x_i$ and the right child of $x_i$. Suppose without loss of generality that the unique path leading to $T'(\boldsymbol{x}) = 1$ includes the left child of $x_i$ (i.e. $T'_l(\boldsymbol{x}) = 1$). By construction,

$$\begin{aligned} s(\boldsymbol{x}, T') = \{t_l \wedge t_r : t_l \in s(\boldsymbol{x}, T'_l), t_r \in s(\boldsymbol{x}, T'_r)\} \\ \cup \{l_i \wedge t_l : t_l \in s(\boldsymbol{x}, T'_l)\} \end{aligned}$$

where $l_i = \overline{x}_i$ if $x_i = 0$ in $\boldsymbol{x}$, and $l_i = x_i$ otherwise. Since by induction hypothesis $s(\boldsymbol{x}, T'_l) = s(\boldsymbol{x}, T'_r) = \sigma(\boldsymbol{x}, d)$, it follows that $\sigma(\boldsymbol{x}, d+1) = \sigma(\boldsymbol{x}, d)^2 + \sigma(\boldsymbol{x}, d)$. Finally, since the doubly exponential sequence[8] given by $a(1) = 1$ and $a(d+1) = a(d)^2 + a(d)$ satisfies $a(d) = \lfloor c^{2^{d-1}} \rfloor$, where $c \sim 1.59791$, it follows that $\sigma(\boldsymbol{x}, k) \geq \lfloor (3/2)^{2^{k-1}} \rfloor$. Using $2^{k-1} = (n+1)/2$, we get the desired result. □

## Proof of Proposition 3

*Proof.* Let $\boldsymbol{x}^*$ be a solution of $(C_{\text{soft}}, C_{\text{hard}})$. Observe that the set of all hard clauses $c_{|\boldsymbol{x}}$ (where $c$ is a clause of $\mathtt{CNF}(T)$) is a monotone set of clauses. Especially, the literals that occur in the set always have the same polarity. Thus in order to satisfy such a clause $c_{|\boldsymbol{x}}$, $\boldsymbol{x}^*$ must set a literal $\ell$ of $t_{\boldsymbol{x}}$ to 1. Thus, $\boldsymbol{x}^*$ satisfies all the hard clauses of the instance if and only if the term consisting of the literals that are shared by $t_{\boldsymbol{x}} = \bigwedge_{i=1}^n \ell_i$ and $t_{\boldsymbol{x}^*}$ is an implicant of $T$ and is implied by $\boldsymbol{x}$.

Finally, the soft clauses of $C_{\text{soft}}$ are used to select among the assignments that satisfy all the hard clauses, the ones that correspond to minimal reasons. Soft clauses are given by literals $\ell_i$, which are precisely the complementary literals to those occurring in $t_{\boldsymbol{x}}$. Having such a soft clause $\ell_i$ violated by $\boldsymbol{x}^*$ means that the literal $\overline{\ell}$ of $t_{\boldsymbol{x}}$ is necessary to get an implicant of $T$ given the assignment of the other variables in $\boldsymbol{x}^*$. Whenever a soft clause $\ell_i$ is violated by $\boldsymbol{x}^*$ a penalty of 1 incurs. This ensures that the term consisting of the literals that are shared by $t_{\boldsymbol{x}} = \bigwedge_{i=1}^n \ell_i$ and $t_{\boldsymbol{x}^*}$ is a minimal reason for $\boldsymbol{x}$ given $F$. □

[8] See https://oeis.org/A007018.

## Proof of Proposition 4

*Proof.* Given $T \in \texttt{DT}_n$, and $\boldsymbol{x} \in \{0,1\}^n$ such that $T(x) = 1$, recall that $H_{\boldsymbol{x}} = (X, E)$ is the hypergraph such that $X = t_{\boldsymbol{x}}$ and $E = \{c \cap t_{\boldsymbol{x}} : c \in \texttt{CNF}(T)\}$. We only need to show that finding a minimal reason for $\boldsymbol{x}$ given $T$ is equivalent to finding for a minimal hitting set of $H_{\boldsymbol{x}}$. The approximation result directly follows from the performance analysis of the greedy algorithm for MIN SET COVER [Slavík, 1997], which is equivalent to MIN HITTING SET by simply reverting the roles of vertices and hyperedges.

Recall that any term $t$ over $X_n$ is an implicant of $T$ if and only if $t$ hits every clause $c \in \texttt{CNF}(T)$. This together with the fact that $T(\boldsymbol{x}) = 1$ implies that any subterm $t \subseteq t_{\boldsymbol{x}}$ is an implicant of $T$ if and only if $t$ (viewed as a subset of $X$) hits every hyperedge in $E$. Therefore, $t \subseteq t_{\boldsymbol{x}}$ is a shortest implicant of $T$ if and only if $t$ is a minimal hitting set of $H_{\boldsymbol{x}}$. □

## Proof of Proposition 5

*Proof.* The result comes directly from the fact that the language $\texttt{DT}$ of decision trees over a set $\{x_1, \ldots, x_n\}$ of Boolean variables satisfy the **CD** transformation (conditioning) and the **CT** query (model counting) [Koriche *et al.*, 2013]. □
