# Supplementary material for: On the Explanatory Power of Decision Trees
Source: arXiv:2108.05266 source file (2021-09-04)
Supplement: Supplementary file 3 [file appendix.tex]

\newpage

\section*{Proofs}

\noindent {\bf Proof of Proposition \ref{prop:minimalreasonDT}}

\begin{proof}
    We call \textsc{Minimal Reason} the problem that asks, given $T \in \dt_n$, $\vec x \in \{0,1\}^n$ with $T(x) = 1$ and $k \in \mathbb N$,
    whether there is an implicant $t$ of $T$ of size at most $k$ that covers $\vec x$.  
%    By showing that \textsc{Minimal Reason} is \textsf{NP}-complete, we immediately get the result of Proposition \ref{prop:minimalreasonDT}.
%
%    The membership of \textsc{Minimal Reason} to \textsf{NP} is decided by the following nondeterministic procedure: 
%    on input $T$, $\vec x$ with $T(\vec x) = 1$ and $k$, guess a subset $t$ of $t_{\vec x}$ such that $\size{t} \leq k$, 
%    and check in $\mathcal O(\size{T} + \size{t})$ time whether $t$ is an implicant of $T$. 
    
    Our objective is to prove that \textsc{Minimal Reason} is {\sf NP}-hard. 
    To this end, let us first recall that a \emph{vertex cover} of an undirected graph $G = (X,E)$
    is a subset $V \subseteq X$ of vertices such that $\{y,z\} \cap V \neq \emptyset$ for 
    every edge $e = \{y,z\}$ in $E$. In the \textsc{Min Vertex Cover} problem, we are given a graph $G$ together with an integer 
    $k \in \mathbb N$, and the task is to find a vertex cover $V$ of $G$ of size at most $k$. 
    \textsc{Min Vertex Cover} is a well-known {\sf NP}-hard problem \cite{Karp1972}, 
    and we now show that it can be reduced in polynomial time to \textsc{Minimal Reason}.

    Suppose that we are given a graph $G = (X,E)$ and assume, without loss of generality, that $G$ does not include isolated vertices.  
    For any $y \in X$, let $E_y = \{e \in E: y \in e\}$ denote the set of edges in $G$ that are adjacent to $y$, 
    and let $N_y = \{z \in X: \{y,z\} \in E\}$ denote the set of neighbors of $y$ in $G$.
    By $G \setminus y$, we denote the deletion of $y$ from $G$, obtained by removing $y$ and its adjacent edges, 
    i.e., $G \setminus y = (X \setminus \{y\}, E \setminus E_y)$. 
    We associate with $G$ a decision tree $T(G)$ over $X_n = X$ using the following recursive algorithm.
    If $G$ is the empty graph (i.e. $E = \emptyset$), then return the decision tree rooted at a $1$-leaf.
    Otherwise, pick a node $y \in X$ and generate a decision tree $T(G)$ such that:
    \begin{enumerate}
        \item[(1)] the root is labeled by $y$;
        \item[(2)] the left child is the decision tree encoding the monomial $\bigwedge N_y$;
        \item[(3)] the right child is the decision tree $T(G')$ returned by calling the algorithm on $G' = G \setminus y$.
    \end{enumerate}
    By construction, $T(G)$ is a complete backtrack search tree of the formula 
    $\cnf(E) = \bigwedge \{(y \lor z): \{y,z\} \in E\}$, 
    which implies that $T(G)$ and $\cnf(E)$ are logically equivalent.
    Furthermore, $T(G)$ is a comb-shaped tree since recursion only on the rightmost branch. 
    In particular, the algorithm runs in $\mathcal O(n \size{E})$ time, since step (1) takes $\mathcal O(1)$ time, step (2) takes 
    $\mathcal O(n)$ time, and step (3) is called at most $\size{E}$ times. 
    
    Now, with an instance $\vec P_1 = (G,k)$ of \textsc{Min Vertex Cover}, 
    we associate the instance $\vec P_2 = (T(G),\vec x,k)$ of \textsc{Minimal Reason}, where $\vec x = (1,\cdots,1)$. 
    Based on the above algorithm, $\vec P_2$ can be constructed in time polynomial in the size of $\vec P_1$.
    
    Let $V$ be a solution of $\vec P_1$. Since $V$ is a vertex cover of $G$, the term $t_V = \bigwedge V$ 
    is an implicant of the formula $\cnf(E)$.
    Since $t_V \subseteq t_{\vec x}$ and $\size{t_V} \leq k$, it follows from the fact that $\cnf(E)$ and $T(G)$ are 
    logically equivalent that $t_V$ is a solution of $\vec P_2$.  

    Conversely, let $t$ be a solution of $\vec P_2$. Since $t$ is an implicant of $T(G)$, it follows that $t$ is an implicant 
    of $\cnf(E)$. This together with the fact that $t \subseteq t_{\vec x}$ implies that the subset of vertices 
    $V \subseteq X_n$, satisfying $\bigwedge V = t$, is a vertex cover of $G$. Since $\size V \leq k$, it is therefore a solution of $\vec P_1$.

\end{proof}

\noindent {\bf Proof of Proposition \ref{prop:nbDT}}

\begin{proof}
    Let $T$ be the complete binary tree of depth $k$, formed by $n = 2^k - 1$ internal nodes and $2^k$ leaves. We assume a breadth-first ordering of internal nodes, 
    such that the root is labeled by $x_1$, the nodes of depth $1$ are labeled by $x_2$ and $x_3$, and so on. For an arbitrary instance $\vec x \in \{0,1\}^n$ and any 
    complete subtree $T'$ of $T$ of depth $d$, let $s(\vec x,T')$ denote the set of sufficient reasons of $\vec x$ given $T'$, and 
    let $\sigma(\vec x,d) = \size{s(\vec x,T')}$  denote the number of those sufficient reasons. We show by induction on $d$ that:
    \begin{align}
        \sigma(\vec x, 1) &= 1 \label{prop:nbDT:base}\\
        \sigma(\vec x, d + 1) &= \sigma(\vec x,d)(\sigma(\vec x,d) + 1) \label{prop:nbDT:induction}
    \end{align}
    For the base case (\ref{prop:nbDT:base}), any complete subtree $T'$ of $T$ of depth $d = 1$ has a single internal node, say $x_i$, with two leaves 
    labeled by $0$ and $1$, respectively. Therefore, the unique sufficient reason for $\vec x$ given $T'$ is either $x_i$ or $\overline x_i$, and hence,
    $\sigma(\vec x, 1) = 1$. Now, consider any complete subtree $T'$ of $T$ of depth $d + 1$ rooted at a node $x_i$. Let $T'_l(x_i)$ and $T'_r(x_i)$
    denote the subtrees of depth $d$, respectively rooted at the left child of $x_i$ and the right child of $x_i$. Suppose without loss of generality 
    that the unique path leading to $T'(\vec x) = 1$ includes the left child of $x_i$ (i.e. $T'_l(\vec x) = 1$). By construction, 
    \begin{align*}
        s(\vec x, T') = \{t_l \land t_r: t_l \in s(\vec x, T'_l), t_r \in s(\vec x, T'_r)\} \\
         \cup \{l_i \land t_l: t_l \in s(\vec x, T'_l)\} 
    \end{align*}
    where $l_i = \overline x_i$ if $x_i = 0$ in $\vec x$, and $l_i = x_i$ otherwise. Since by induction hypothesis $s(\vec x, T'_l) = s(\vec x, T'_r) = \sigma(\vec x,d)$, 
    it follows that $\sigma(\vec x, d + 1) = \sigma(\vec x,d)^2 + \sigma(\vec x,d)$. Finally, since the doubly exponential sequence\footnote{See \url{https://oeis.org/A007018}.} 
    given by $a(1) = 1$ and $a(d+1) = a(d)^2 + a(d)$ satisfies  $a(d) = \lfloor c^{2^{d-1}} \rfloor$, where $c \sim 1.59791$, it follows that 
    $\sigma(\vec x, k) \geq \lfloor (\nicefrac{3}{2})^{2^{k-1}} \rfloor$. Using $2^{k-1} = (n + 1)/2$, we get the desired result.   
\end{proof}

\noindent {\bf Proof of Proposition \ref{prop:minimaloptim}}
\begin{proof}
Let $\vec x^*$ be a solution of $(C_{\mathrm{soft}}, C_{\mathrm{hard}})$.
Observe that the set of all hard clauses $c_{\mid \vec x}$ (where $c$ is a clause of $\cnf(T)$) is a 
monotone set of clauses. Especially, the literals that occur in the set always have the same polarity. Thus in order to satisfy
such a clause $c_{\mid \vec x}$, $\vec x^*$ must set a literal $\ell$ of $t_{\vec x}$ to $1$. 
Thus, $\vec x^*$ satisfies all the hard clauses of the instance if and only if the term consisting of the literals that 
are shared by $t_{\vec x} = \bigwedge_{i=1}^n \ell_i$ and  $t_{\vec x^*}$ is an implicant of $T$ and is implied by $\vec x$.

%Finally, the soft clauses $\{(\overline{x_i}, w(x_i)) \mid x_i(\vec x) = 1\} \cup \{(x_i, w(x_i)) \mid x_i(\vec x) = 0\}$ are used to
Finally, the soft clauses of $C_{\mathrm{soft}}$ %\{\overline{x_i} \mid x_i(\vec x) = 1\} \cup \{x_i, \mid x_i(\vec x) = 0\}$ 
are used to select among the assignments that satisfy all the hard clauses, the ones that correspond to minimal reasons.
Soft clauses are given by literals $\ell_i$, which are precisely the complementary literals to those occurring in $t_{\vec x}$.
Having such a soft clause $\ell_i$ violated by $\vec x^*$ means that the literal $\overline{\ell}$ of $t_{\vec x}$ is necessary to get
an implicant of $T$ given the assignment of the other variables in $\vec x^*$. Whenever a soft clause $\ell_i$ is violated by $\vec x^*$
%a penalty corresponding to the weight of the variable of $\ell_i$ incurs. This ensures that  the term consisting of the literals 
a penalty of $1$ incurs. This ensures that  the term consisting of the literals 
that are shared by $t_{\vec x} = \bigwedge_{i=1}^n \ell_i$ and  $t_{\vec x^*}$ is a minimal reason for $\vec x$ given $F$.
%a minimal-weight reason for $\vec x$ given $F$ and $w$.
\end{proof}

\noindent {\bf Proof of Proposition \ref{prop:approximable}}

\begin{proof}
    Given $T \in \dt_n$, and $\vec x \in \{0,1\}^n$ such that $T(x) = 1$, recall that $H_{\vec x} = (X,E)$ is the hypergraph
    such that $X = t_{\vec x}$ and $E = \{c \cap t_{\vec x}: c \in \cnf(T)\}$. We only need to show that finding a minimal 
    reason for $\vec x$ given $T$ is equivalent to finding for a minimal hitting set of $H_{\vec x}$. The approximation result 
    directly follows from the performance analysis of the greedy algorithm for \textsc{Min Set Cover} \cite{SLAVIK1997}, 
    which is equivalent to \textsc{Min Hitting Set} by simply reverting the roles of vertices and hyperedges.  
    
    Recall that any term $t$ over $X_n$ is an implicant of $T$ if and only if $t$ hits every clause $c \in \cnf(T)$.
    This together with the fact that $T(\vec x) = 1$ implies that any subterm $t \subseteq t_{\vec x}$ is an 
    implicant of $T$ if and only if $t$ (viewed as a subset of $X$) hits every hyperedge in $E$. 
    Therefore, $t \subseteq t_{\vec x}$ is a shortest implicant of $T$ if and only if $t$ is a minimal hitting set of 
    $H_{\vec x}$. 
\end{proof}

%
%\begin{proof}
%\pierre{TBW}
%\end{proof}

\noindent {\bf Proof of Proposition \ref{prop:probabilisticreasonDT}}

\begin{proof}
The result comes directly from the fact that the language \dt\ of decision trees over a set $\{x_1,$ $\ldots,$ $x_n\}$ of Boolean variables
satisfy the \cd\ transformation (conditioning) and the \ct\ query (model counting) \cite{Koricheetal13}.
\end{proof}
